# Supplementary material for: Electron Dynamics with the Time-Dependent Density Matrix Renormalization Group
Source: arXiv:2010.02049 ancillary file (2021-06-05)
Supplement: Supplementary file 1 [file SupportingInfo.pdf]

# Supporting information for: Electron Dynamics with the Time-Dependent Density Matrix Renormalization Group

Alberto Baiardi*

*ETH Zürich, Laboratorium für Physikalische Chemie, Vladimir-Prelog-Weg 2, 8093 Zürich, Switzerland.*

E-mail: alberto.baiardi@phys.chem.ethz.ch

# 1 Additional information on the charge dynamics in benzene

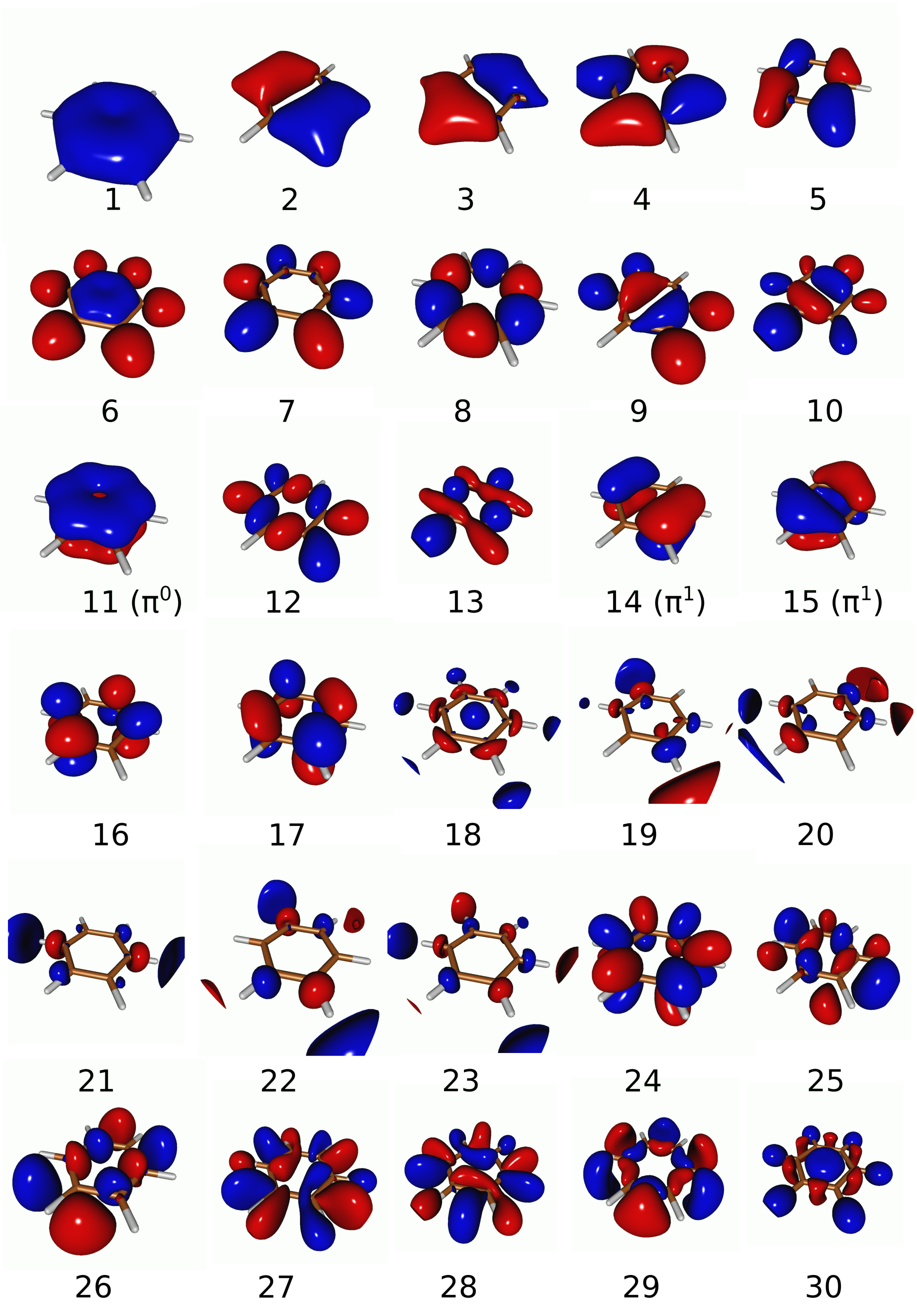


Figure S1: Canonical Hartree-Fock orbital of benzene calculated with the 6-31G* basis set. The ionized orbital (denoted as $\pi^0$ in the main text) is number 11, while the two degenerate $\pi^1$ orbitals are 14 and 15.

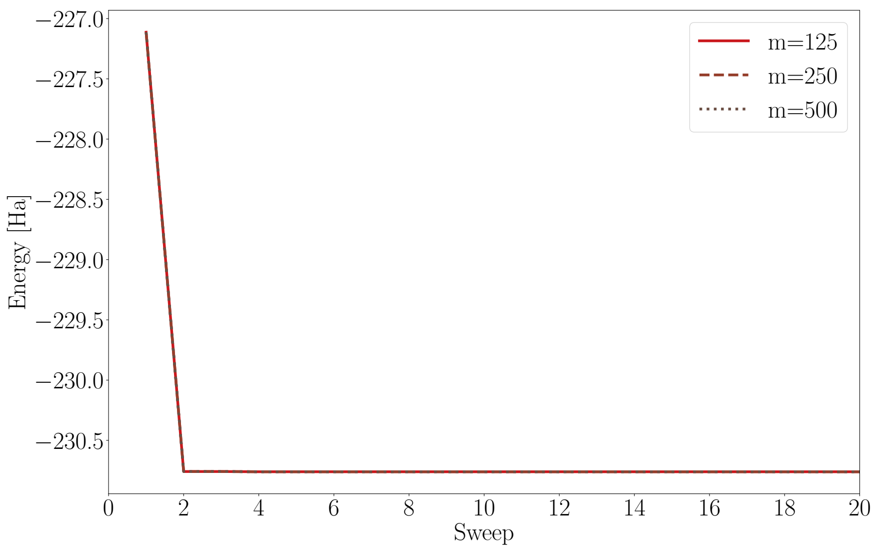


Figure S2: iTD-DMRG(TS) energy convergence of benzene as a function of the sweep number for CAS(14,14).

Table S1: Ground-state iTD-DMRG(TS) energy (in Hartree atomic units) of benzene based on CAS(20,20) and CAS(26,26) and $\Delta t$=500 as.

| | $m$=125 | $m$=250 | $m$=500 | $m$=1000 |
|---|---|---|---|---|
| CAS(20,20) | -230.79250 | -230.79406 | -230.79478 | -230.79510 |
| CAS(26,26) | -230.82680 | -230.83226 | -230.83531 | -230.83724 |

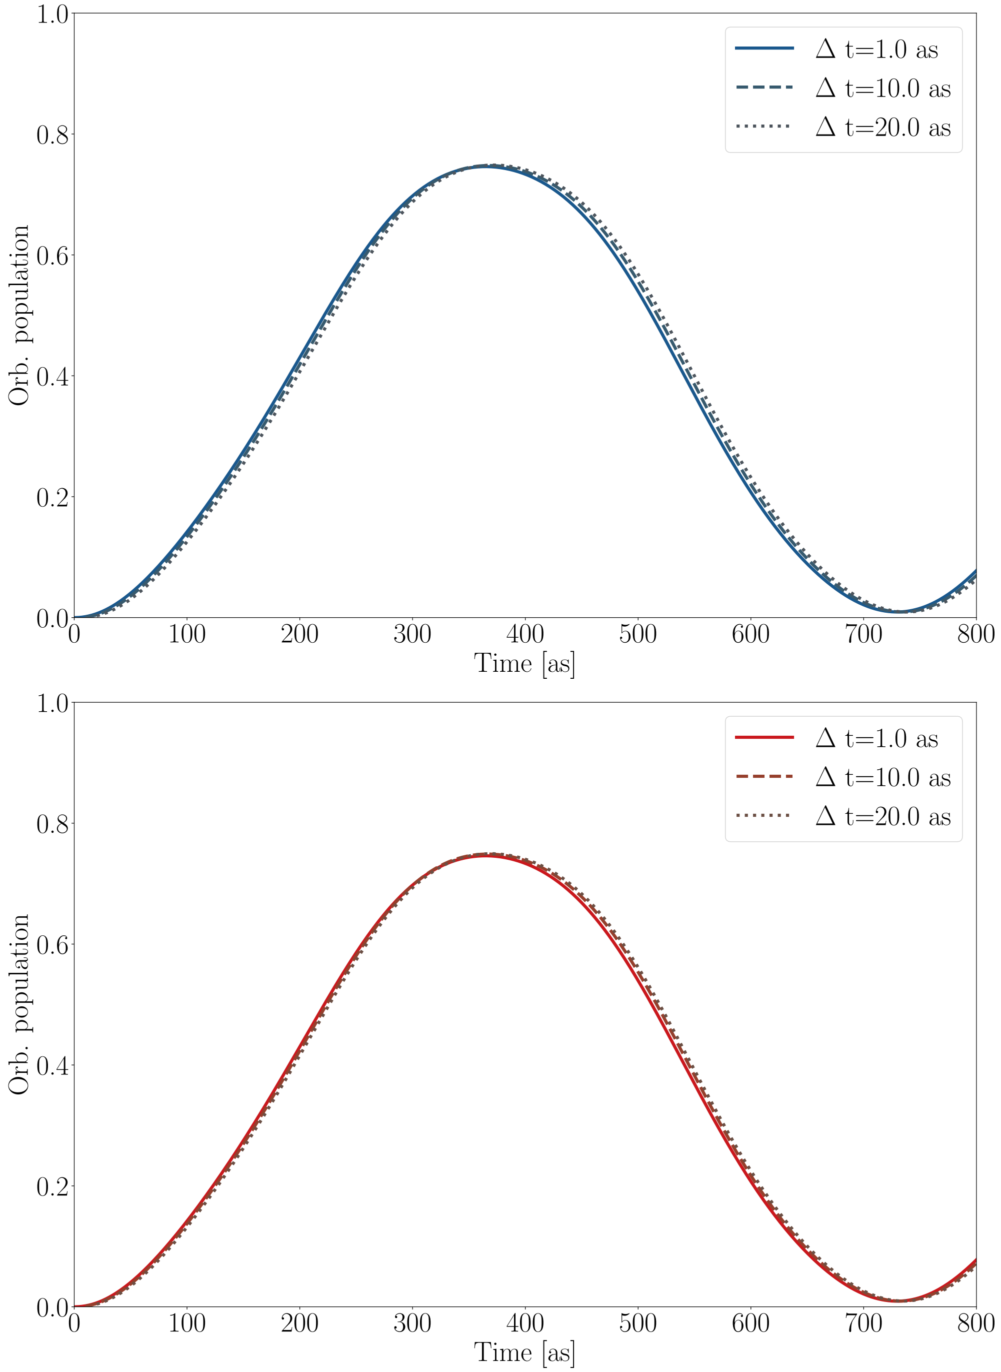


Figure S3: Time evolution of the $\pi^0$ orbital population of benzene following ionization calculated with TD-DMRG(TS), $m$=250 (upper panel) and $m$=500 (lower panel), and varying $\Delta t$ values.

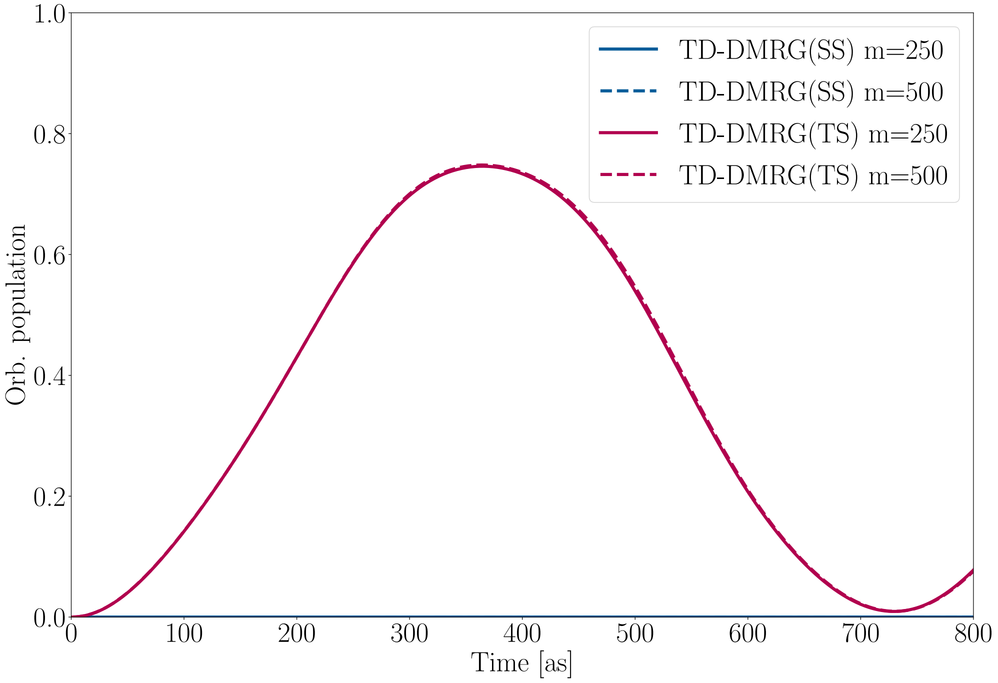


Figure S4: Time evolution of the $\pi^0$ orbital population of benzene following ionization calculated with TD-DMRG(SS) and TD-DMRG(TS) based on CAS(14,14).

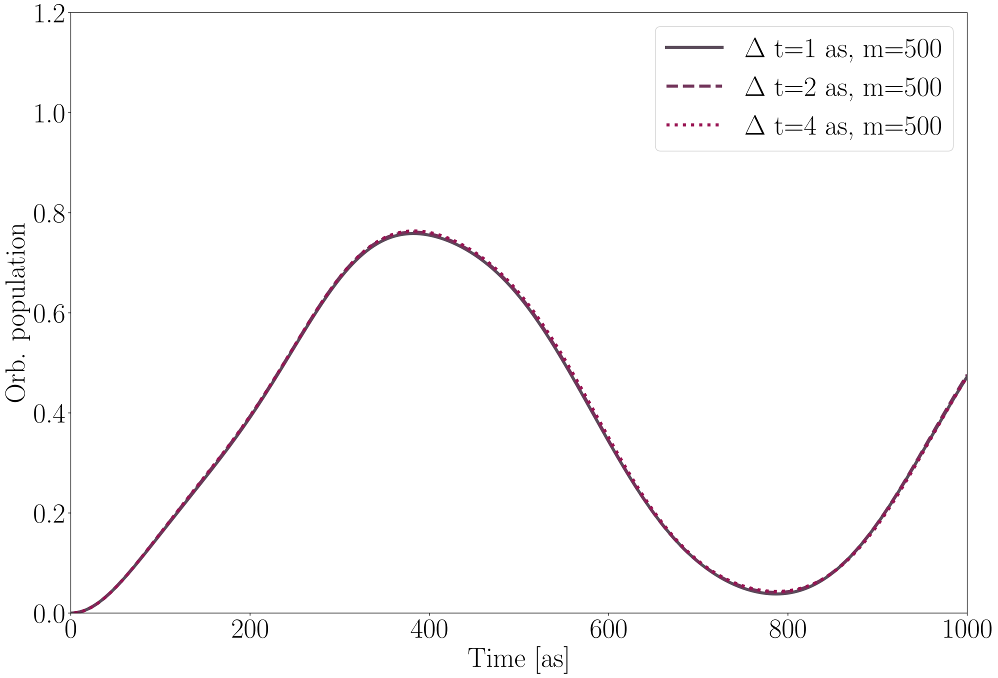


Figure S5: Time evolution of the $\pi^0$ orbital population of benzene following ionization calculated with TD-DMRG(TS), $m$=500, CAS(20,20) and varying integration time steps.

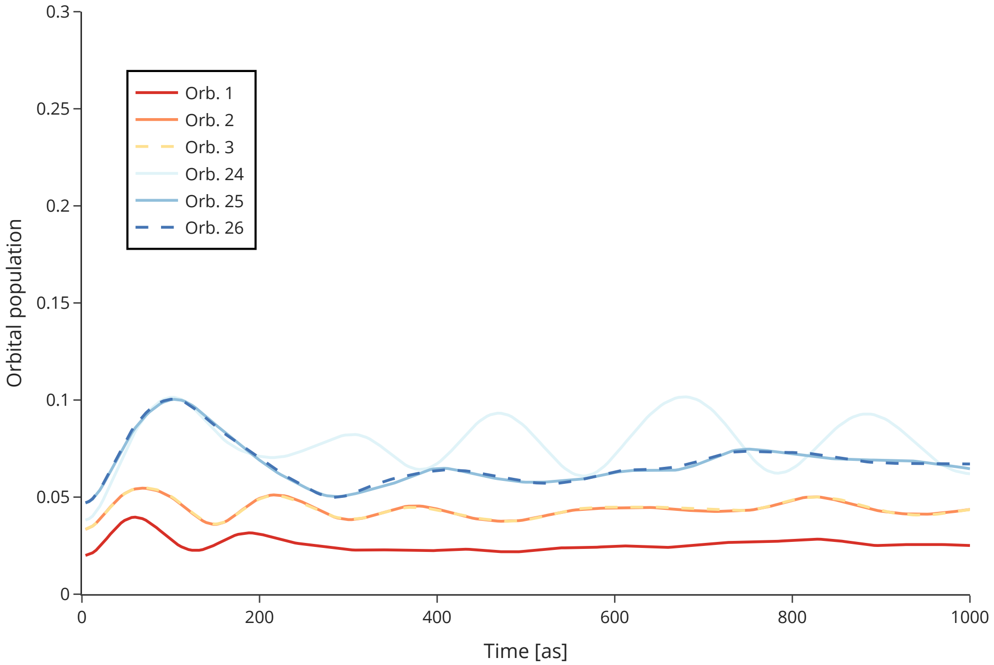


Figure S6: Time evolution of the single-orbital entropy $s^{(1)}$ for the three lowest-energy and three highest-energy orbitals of benzene calculated with TD-DMRG(TS), CAS(26,26), $m$=500, and $\Delta t$=4 as. Orbitals are numbered in increasing energy order.

# 2 Additional information on the absorption spectrum of decacene

Table S2: TI-DMRG ground-state energy of decacene obtained with TI-DMRG and iTD-DMRG for varying $m$ values, based on a CAS(10,10), and with $\Delta t$=100 as.

| | $m$ | SS | TS |
|---|---|---|---|
| TI-DMRG | 125 | -6.95753 | -6.96254 |
| | 250 | -6.96168 | -6.69258 |
| | 500 | -6.96260 | -6.96276 |
| iTD-DMRG | 125 | -6.95662 | -6.96254 |
| | 250 | -6.95934 | -6.96259 |
| | 500 | -6.96245 | -6.96276 |

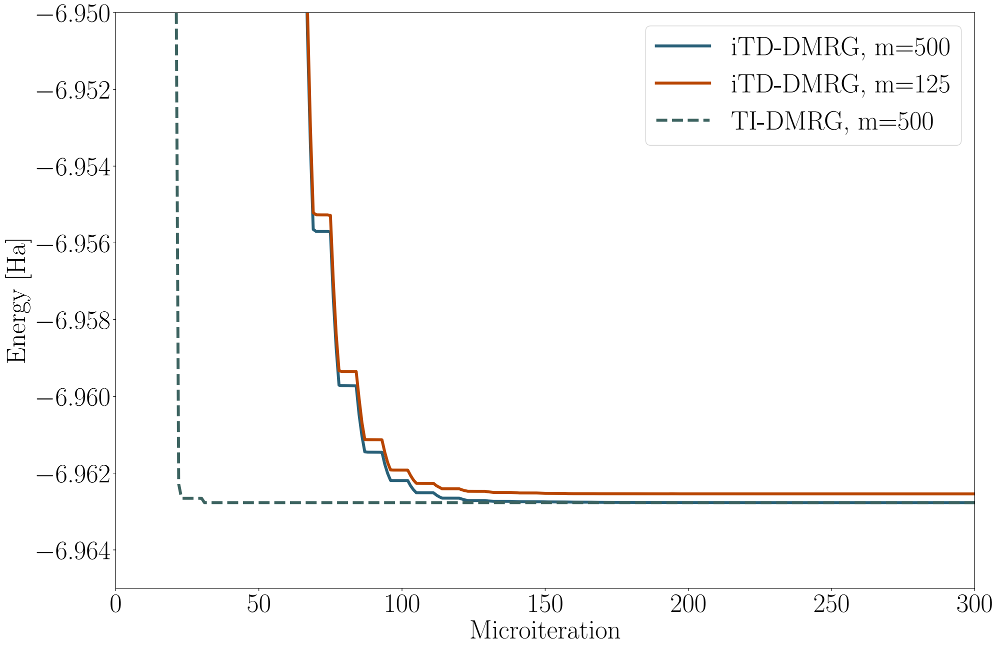


Figure S7: Energy convergence of iTD-DMRG(TS) and TI-DMRG(TS) for decacene obtained with CAS(10,10).

Table S3: TI-DMRG excitation energies ($\Delta E$) and corresponding transition dipole moment ($\boldsymbol{\mu}_{if}$) for the 20 lowest-energy excited states of decacene calculated with TI-DMRG.

| Exc. state | $m$=125 | | $m$=250 | |
|---|---|---|---|---|
| | $\Delta E$ | $\mu_{if}$ | $\Delta E$ | $\mu_{if}$ |
| 1 | 1.63582 | 6.02171E-14 | 1.63383 | 5.51467E-17 |
| 2 | 2.38911 | 2.61717E+00 | 2.39070 | 1.05122E+00 |
| 3 | 2.47704 | -1.32077E-06 | 2.47640 | 1.29649E-12 |
| 4 | 3.23992 | 6.09734E-06 | 3.24004 | 1.14525E-05 |
| 5 | 3.32825 | -1.01377E-07 | 3.31985 | -1.64998E-12 |
| 6 | 3.33878 | -4.60182E-06 | 3.33891 | 7.29552E-07 |
| 7 | 3.53275 | 3.84359E-06 | 3.52731 | 1.07960E-12 |
| 8 | 4.02290 | 1.58083E-01 | 4.01616 | -1.05614E+00 |
| 9 | 4.22401 | 8.52178E-09 | 4.21948 | 1.42117E-12 |
| 10 | 4.29937 | 1.94683E-01 | 4.29398 | -3.45847E-01 |
| 11 | 4.38059 | 3.41167E-06 | 4.37644 | -4.47556E-07 |
| 12 | 4.42936 | 1.55454E-07 | 4.42598 | 9.10905E-12 |
| 13 | 4.63958 | -5.85844E-01 | 4.63543 | 6.04199E-01 |
| 14 | 4.78194 | 4.69661E-07 | 4.78075 | -1.64355E-12 |
| 15 | 4.78698 | -3.87481E-08 | 4.78464 | -1.59496E-14 |
| 16 | 4.87515 | 1.26325E-06 | 4.86753 | 2.97413E-06 |
| 17 | 4.98757 | 4.44766E-08 | 4.99037 | -9.03149E-12 |
| 18 | 5.05045 | -1.69439E-06 | 5.03798 | 3.43116E-12 |
| 19 | 5.23338 | 5.31578E-07 | 5.22638 | -2.26406E-06 |
| 20 | 5.31334 | -1.46661E-05 | 5.30834 | 1.10488E-06 |
| 21 | 5.38520 | 9.80675E-07 | 5.37473 | -4.35951E-12 |
| 22 | 5.46552 | 3.32885E-09 | 5.46572 | 1.13020E-11 |
| 23 | 5.48102 | 5.76748E-01 | 5.47345 | -1.18697E-01 |
| 24 | 5.51620 | 5.92789E-01 | 5.50895 | 1.95395E-02 |
| 25 | 5.61063 | -5.99718E-06 | 5.60336 | -5.93805E-06 |
| 26 | 5.72104 | -4.72455E-07 | 5.70603 | -1.94509E-11 |
| 27 | 5.73783 | -9.88420E-06 | 5.82632 | -4.16779E-02 |
| 28 | 5.78463 | 2.93355E-08 | 5.77871 | -4.35863E-03 |
| 29 | 5.78766 | -1.35764E-05 | 5.78144 | 1.61311E-04 |

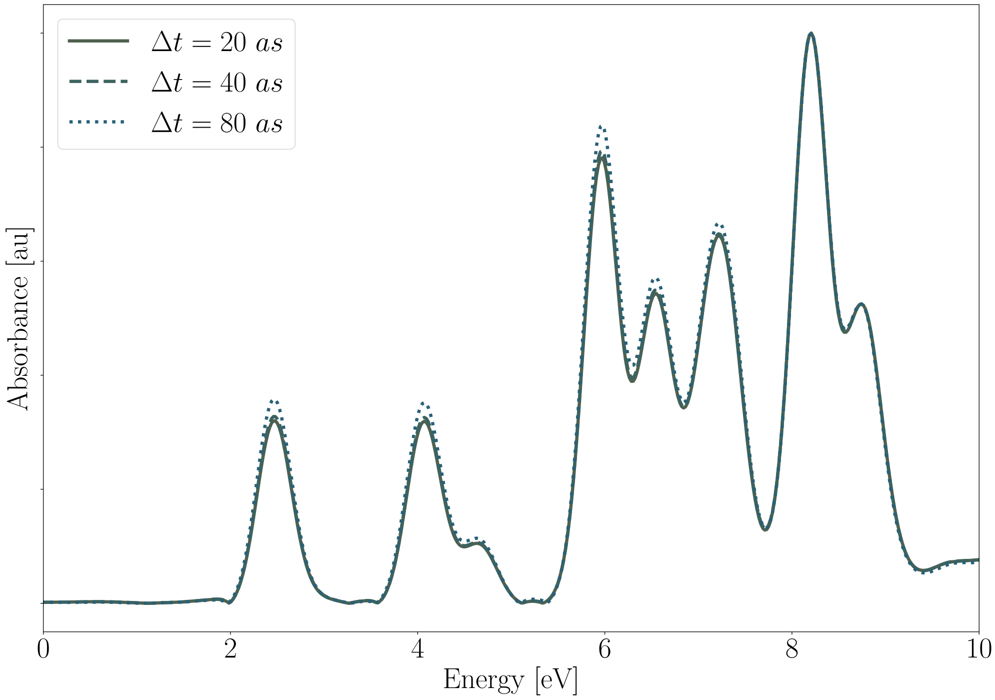


Figure S8: Absorption spectrum of decacene obtained with TD-DMRG(TS) based on CAS(10,10) for different step sizes $\Delta t$ and for $m$=500.

# 3 Additional information on the response properties of BH

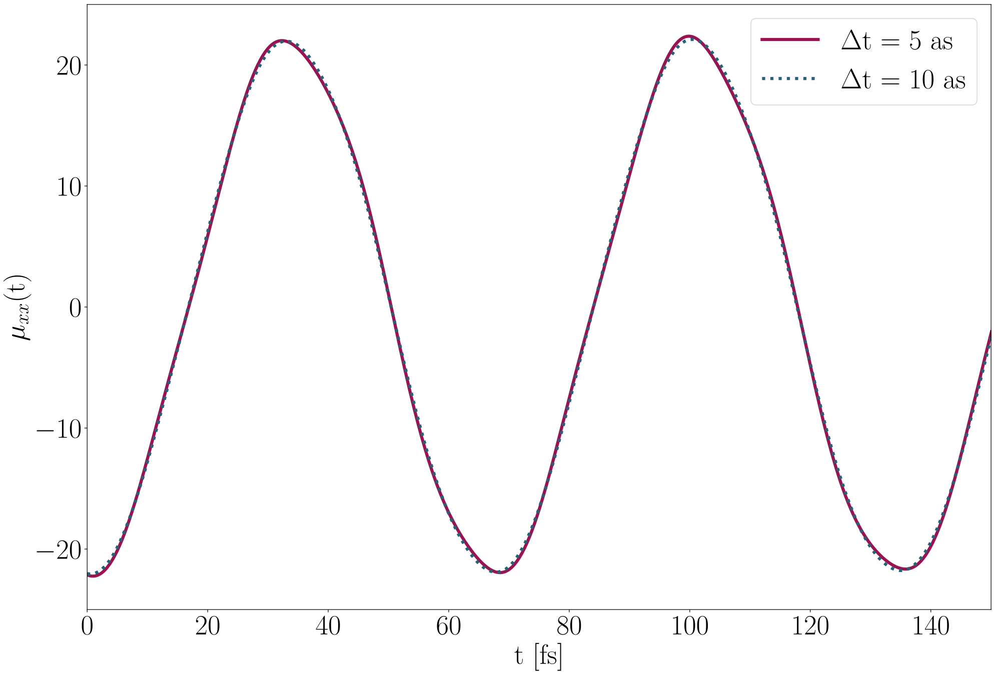


Figure S9: First-order dipole response $\mu_{xx}(t)$ of BH calculated with EMR2-TD-DMRG(SS), with a perturbing field $E_0$ of 0.003 au and the cc-pVDZ basis.

Table S4: Ground-state energy (in Hartree atomic units) of BH calculated with iTD-DMRG(SS) and iTD-DMRG(TS) based on the cc-pVDZ basis both with the non spin-adapted (2U1) and with the spin adapted (SU(2)) DMRG formulations. We also report the results obtained with the larger aug-cc-pVDZ basis and iTD-DMRG(TS).

| | | cc-pVDZ | | aug-cc-pVDZ | |
|---|---|---|---|---|---|
| | | $m$=125 | $m$=250 | $m$=125 | $m$=250 |
| 2U1 | SS | -24.16214 | -24.16214 | - | - |
| | TS | -25.21620 | -25.21621 | -25.21938 | -25.21955 |
| SU(2) | SS | -25.15821 | -25.15822 | - | - |
| | TS | -25.21621 | -25.21621 | -25.21955 | -25.21957 |
